# Supplementary material for: Compositional Neural Textures
Source: arXiv:2404.12509 source file (2024-09-23)
Supplement: Supplementary file 1 [file fig_appendix_ablation_architectures.tex]

\begin{figure*}[b]
	\centering
	\captionsetup[subfigure]{labelformat=empty,justification=centering}
	\begingroup
	\setlength{\tabcolsep}{0pt} 
	
	\begin{tabular}{cc}
	\begin{tabular}{ccccc}
		\subfloat[Input]{
			\includegraphics[width=0.11\linewidth]{figs/results/ablations/01112024/full/img/301_6/img.png}
		}&
		\raisebox{0.25in}{\rotatebox[origin=t]{90}{Gaussian/Seg.}}
		&
		\subfloat[]{
			\includegraphics[width=0.11\linewidth]{figs/results/ablations/01112024/nosegmentation/img/301_6/gaussian.png}
		}&
		\subfloat[]{
			\includegraphics[width=0.11\linewidth]{figs/results/ablations/01112024/nogaussian/img/301_6/seg.png}
		}&
		\subfloat[]{
			\includegraphics[width=0.11\linewidth]{figs/results/ablations/01112024/full/img/301_6/seg.png}
		}\\[-0.8cm]
		&
		\subfloat{
			\raisebox{0.25in}{\rotatebox[origin=t]{90}{Recon.} } 
		}
		&
		\subfloat[]{
			\includegraphics[width=0.11\linewidth]{figs/results/ablations/01112024/nosegmentation/img/301_6/recon.png}
		}&
		\subfloat[]{
			\includegraphics[width=0.11\linewidth]{figs/results/ablations/01112024/nogaussian/img/301_6/recon.png}
		}&
		\subfloat[]{
			\includegraphics[width=0.11\linewidth]{figs/results/ablations/01112024/full/img/301_6/recon.png}
		}\\[-0.8cm]
		\subfloat[]{
			\includegraphics[width=0.11\linewidth]{figs/results/ablations/01112024/full/301_1/texture.png}
		}&
		\raisebox{0.4in}{\multirow{2}{*}{\rotatebox[origin=t]{90}{Texture transfer}}}
		&
		\subfloat[]{
			\includegraphics[width=0.11\linewidth]{figs/results/ablations/01112024/nosegmentation/301_1/0_6.png}
		}&
		\subfloat[]{
			\includegraphics[width=0.11\linewidth]{figs/results/ablations/01112024/nogaussian/301_1/0_6.png}
		}&
		\subfloat[]{
			\includegraphics[width=0.11\linewidth]{figs/results/ablations/01112024/full/301_1/0_6.png}
		}\\[-0.8cm]
		\subfloat[Appearance]{
			\includegraphics[width=0.11\linewidth]{figs/results/ablations/01112024/full/301_17/texture.png}
		}&
		&
		\subfloat[w/o seg.]{
			\includegraphics[width=0.11\linewidth]{figs/results/ablations/01112024/nosegmentation/301_17/0_6.png}
		}&
		\subfloat[w/o Gauss.]{
			\includegraphics[width=0.11\linewidth]{figs/results/ablations/01112024/nogaussian/301_17/0_6.png}
		}&
		\subfloat[Full]{
			\includegraphics[width=0.11\linewidth]{figs/results/ablations/01112024/full/301_17/0_6.png}
		}\\
		\subfloat[Input]{
			\includegraphics[width=0.11\linewidth]{figs/results/ablations/01112024/full/img/301_9/img.png}
		}&
		\raisebox{0.25in}{\rotatebox[origin=t]{90}{Gaussian/Seg.}}
		&
		\subfloat[]{
			\includegraphics[width=0.11\linewidth]{figs/results/ablations/01112024/nosegmentation/img/301_9/gaussian.png}
		}&
		\subfloat[]{
			\includegraphics[width=0.11\linewidth]{figs/results/ablations/01112024/nogaussian/img/301_9/seg.png}
		}&
		\subfloat[]{
			\includegraphics[width=0.11\linewidth]{figs/results/ablations/01112024/full/img/301_9/seg.png}
		}\\[-0.8cm]
		&
		\subfloat{
			\raisebox{0.25in}{\rotatebox[origin=t]{90}{Recon.} } 
		}
		&
		\subfloat[]{
			\includegraphics[width=0.11\linewidth]{figs/results/ablations/01112024/nosegmentation/img/301_9/recon.png}
		}&
		\subfloat[]{
			\includegraphics[width=0.11\linewidth]{figs/results/ablations/01112024/nogaussian/img/301_9/recon.png}
		}&
		\subfloat[]{
			\includegraphics[width=0.11\linewidth]{figs/results/ablations/01112024/full/img/301_9/recon.png}
		}\\[-0.8cm]
		\subfloat[]{
			\includegraphics[width=0.11\linewidth]{figs/results/ablations/01112024/full/301_1/texture.png}
		}&
		\raisebox{0.4in}{\multirow{2}{*}{\rotatebox[origin=t]{90}{Texture transfer}}}
		&
		\subfloat[]{
			\includegraphics[width=0.11\linewidth]{figs/results/ablations/01112024/nosegmentation/301_1/0_9.png}
		}&
		\subfloat[]{
			\includegraphics[width=0.11\linewidth]{figs/results/ablations/01112024/nogaussian/301_1/0_9.png}
		}&
		\subfloat[]{
			\includegraphics[width=0.11\linewidth]{figs/results/ablations/01112024/full/301_1/0_9.png}
		}\\[-0.8cm]
		\subfloat[Appearance]{
			\includegraphics[width=0.11\linewidth]{figs/results/ablations/01112024/full/301_17/texture.png}
		}&
		&
		\subfloat[w/o seg.]{
			\includegraphics[width=0.11\linewidth]{figs/results/ablations/01112024/nosegmentation/301_17/0_9.png}
		}&
		\subfloat[w/o Gauss.]{
			\includegraphics[width=0.11\linewidth]{figs/results/ablations/01112024/nogaussian/301_17/0_9.png}
		}&
		\subfloat[Full]{
			\includegraphics[width=0.11\linewidth]{figs/results/ablations/01112024/full/301_17/0_9.png}
		}\\
	\end{tabular}
	\begin{tabular}{ccccc}
		\subfloat[Input]{
			\includegraphics[width=0.11\linewidth]{figs/results/ablations/01112024/full/img/301_12/img.png}
		}&
		\raisebox{0.25in}{\rotatebox[origin=t]{90}{Gaussian/Seg.}}
		&
		\subfloat[]{
			\includegraphics[width=0.11\linewidth]{figs/results/ablations/01112024/nosegmentation/img/301_12/gaussian.png}
		}&
		\subfloat[]{
			\includegraphics[width=0.11\linewidth]{figs/results/ablations/01112024/nogaussian/img/301_12/seg.png}
		}&
		\subfloat[]{
			\includegraphics[width=0.11\linewidth]{figs/results/ablations/01112024/full/img/301_12/seg.png}
		}\\[-0.8cm]
		&
		\subfloat{
			\raisebox{0.25in}{\rotatebox[origin=t]{90}{Recon.} } 
		}
		&
		\subfloat[]{
			\includegraphics[width=0.11\linewidth]{figs/results/ablations/01112024/nosegmentation/img/301_12/recon.png}
		}&
		\subfloat[]{
			\includegraphics[width=0.11\linewidth]{figs/results/ablations/01112024/nogaussian/img/301_12/recon.png}
		}&
		\subfloat[]{
			\includegraphics[width=0.11\linewidth]{figs/results/ablations/01112024/full/img/301_12/recon.png}
		}\\[-0.8cm]
		&
		\raisebox{0.4in}{\multirow{2}{*}{\rotatebox[origin=t]{90}{Texture transfer}}}
		&
		\subfloat[]{
			\includegraphics[width=0.11\linewidth]{figs/results/ablations/01112024/nosegmentation/301_1/0_12.png}
		}&
		\subfloat[]{
			\includegraphics[width=0.11\linewidth]{figs/results/ablations/01112024/nogaussian/301_1/0_12.png}
		}&
		\subfloat[]{
			\includegraphics[width=0.11\linewidth]{figs/results/ablations/01112024/full/301_1/0_12.png}
		}\\[-0.8cm]
		&
		&
		\subfloat[w/o seg.]{
			\includegraphics[width=0.11\linewidth]{figs/results/ablations/01112024/nosegmentation/301_17/0_12.png}
		}&
		\subfloat[w/o Gauss.]{
			\includegraphics[width=0.11\linewidth]{figs/results/ablations/01112024/nogaussian/301_17/0_12.png}
		}&
		\subfloat[Full]{
			\includegraphics[width=0.11\linewidth]{figs/results/ablations/01112024/full/301_17/0_12.png}
		}\\
		\subfloat[Input]{
			\includegraphics[width=0.11\linewidth]{figs/results/ablations/01112024/full/img/301_14/img.png}
		}&
		\raisebox{0.25in}{\rotatebox[origin=t]{90}{Gaussian/Seg.}}
		&
		\subfloat[]{
			\includegraphics[width=0.11\linewidth]{figs/results/ablations/01112024/nosegmentation/img/301_14/gaussian.png}
		}&
		\subfloat[]{
			\includegraphics[width=0.11\linewidth]{figs/results/ablations/01112024/nogaussian/img/301_14/seg.png}
		}&
		\subfloat[]{
			\includegraphics[width=0.11\linewidth]{figs/results/ablations/01112024/full/img/301_14/seg.png}
		}\\[-0.8cm]
		&
		\subfloat{
			\raisebox{0.25in}{\rotatebox[origin=t]{90}{Recon.} } 
		}
		&
		\subfloat[]{
			\includegraphics[width=0.11\linewidth]{figs/results/ablations/01112024/nosegmentation/img/301_14/recon.png}
		}&
		\subfloat[]{
			\includegraphics[width=0.11\linewidth]{figs/results/ablations/01112024/nogaussian/img/301_14/recon.png}
		}&
		\subfloat[]{
			\includegraphics[width=0.11\linewidth]{figs/results/ablations/01112024/full/img/301_14/recon.png}
		}\\[-0.8cm]
		&
		\raisebox{0.4in}{\multirow{2}{*}{\rotatebox[origin=t]{90}{Texture transfer}}}
		&
		\subfloat[]{
			\includegraphics[width=0.11\linewidth]{figs/results/ablations/01112024/nosegmentation/301_1/0_14.png}
		}&
		\subfloat[]{
			\includegraphics[width=0.11\linewidth]{figs/results/ablations/01112024/nogaussian/301_1/0_14.png}
		}&
		\subfloat[]{
			\includegraphics[width=0.11\linewidth]{figs/results/ablations/01112024/full/301_1/0_14.png}
		}\\[-0.8cm]
		&
		&
		\subfloat[w/o seg.]{
			\includegraphics[width=0.11\linewidth]{figs/results/ablations/01112024/nosegmentation/301_17/0_14.png}
		}&
		\subfloat[w/o Gauss.]{
			\includegraphics[width=0.11\linewidth]{figs/results/ablations/01112024/nogaussian/301_17/0_14.png}
		}&
		\subfloat[Full]{
			\includegraphics[width=0.11\linewidth]{figs/results/ablations/01112024/full/301_17/0_14.png}
		}\\
	\end{tabular}
	\end{tabular}
	\endgroup
	\Caption{Ablation studies on network components.}{%
		We visualize the Gaussians/segmentation masks, reconstruction and texture transfer results given appearance-providing textures.
	}%
	\label{fig:appendix:ablation_networks0}
\end{figure*}
