# Supplementary material for: Compositional Neural Textures
Source: arXiv:2404.12509 source file (2024-09-23)
Supplement: Supplementary file 3 [file fig_appendix_dataset_samples1.tex]

\begin{figure}[h]

\centering
\captionsetup[subfigure]{labelformat=empty}

    \foreach \n in {40,...,44}{
        \includegraphics[width=0.19\linewidth]{figs/results/appendix/data_samples/\n.png}%
    }

    \foreach \n in {45,...,49}{
        \includegraphics[width=0.19\linewidth]{figs/results/appendix/data_samples/\n.png}%
    }

    \foreach \n in {50,...,54}{
        \includegraphics[width=0.19\linewidth]{figs/results/appendix/data_samples/\n.png}%
    }

    \foreach \n in {55,...,59}{
        \includegraphics[width=0.19\linewidth]{figs/results/appendix/data_samples/\n.png}%
    }

    \foreach \n in {60,...,64}{
        \includegraphics[width=0.19\linewidth]{figs/results/appendix/data_samples/\n.png}%
    }

    \foreach \n in {65,...,69}{
        \includegraphics[width=0.19\linewidth]{figs/results/appendix/data_samples/\n.png}%
    }

    \foreach \n in {70,...,74}{
        \includegraphics[width=0.19\linewidth]{figs/results/appendix/data_samples/\n.png}%
    }

    \foreach \n in {75,...,79}{
        \includegraphics[width=0.19\linewidth]{figs/results/appendix/data_samples/\n.png}%
    }

    \foreach \n in {80,...,84}{
        \includegraphics[width=0.19\linewidth]{figs/results/appendix/data_samples/\n.png}%
    }

    \foreach \n in {85,...,89}{
        \includegraphics[width=0.19\linewidth]{figs/results/appendix/data_samples/\n.png}%
    }

    \foreach \n in {90,...,94}{
        \includegraphics[width=0.19\linewidth]{figs/results/appendix/data_samples/\n.png}%
    }

    \foreach \n in {95,...,99}{
        \includegraphics[width=0.19\linewidth]{figs/results/appendix/data_samples/\n.png}%
    }

    \foreach \n in {35,...,39}{
        \includegraphics[width=0.19\linewidth]{figs/results/appendix/data_samples/\n.png}%
    }

\Caption{Continuation of \Cref{fig:dataset_samples}.}
{%
    
}
\label{fig:dataset_samples1}
\end{figure}
