# Supplementary material for: Compositional Neural Textures
Source: arXiv:2404.12509 source file (2024-09-23)
Supplement: Supplementary file 4 [file fig_appendix_transfer_by_replace.tex]

\begin{figure*}%
	\centering
	\captionsetup[subfigure]{labelformat=empty}%
	\captionsetup[subfloat]{justification=centering}

	\subfloat[]{%
		\includegraphics[width=0.185\linewidth]{figs/results/appendix/texture_transfer/img/1201_0/img.png}
	}%
	\subfloat[]{%
		\includegraphics[width=0.185\linewidth]{figs/results/appendix/texture_transfer/img/1201_5/img.png}
	}%
	\subfloat[]{%
		\includegraphics[width=0.185\linewidth]{figs/results/appendix/texture_transfer/replace/paper/1201_5/0_0.png}
	}%
	\subfloat[]{%
		\includegraphics[width=0.185\linewidth]{figs/results/appendix/texture_transfer/mean/paper/1201_5/0_0.png}
	}%
	\subfloat[]{%
		\includegraphics[width=0.185\linewidth]{figs/results/appendix/texture_transfer/img/1201_0/seg.png}
	}%

	\vspace{-0.8cm}%
	
	\subfloat[]{%
		\includegraphics[width=0.185\linewidth]{figs/results/appendix/texture_transfer/img/1200_0/img.png}
	}%
	\subfloat[]{%
		\includegraphics[width=0.185\linewidth]{figs/results/appendix/texture_transfer/img/1200_9/img.png}
	}%
	\subfloat[]{%
		\includegraphics[width=0.185\linewidth]{figs/results/appendix/texture_transfer/replace/paper/1200_9/0_0.png}
	}%
	\subfloat[]{%
		\includegraphics[width=0.185\linewidth]{figs/results/appendix/texture_transfer/mean/paper/1200_9/0_0.png}
	}%
	\subfloat[]{%
		\includegraphics[width=0.185\linewidth]{figs/results/appendix/texture_transfer/img/1200_0/seg.png}
	}%

	\vspace{-0.8cm}%
	
	\subfloat[]{%
		\includegraphics[width=0.185\linewidth]{figs/results/appendix/texture_transfer/img/1202_3/img.png}
	}%
	\subfloat[]{%
		\includegraphics[width=0.185\linewidth]{figs/results/appendix/texture_transfer/img/1202_2/img.png}
	}%
	\subfloat[]{%
		\includegraphics[width=0.185\linewidth]{figs/results/appendix/texture_transfer/replace/paper/1202_2/0_3.png}
	}%
	\subfloat[]{%
		\includegraphics[width=0.185\linewidth]{figs/results/appendix/texture_transfer/mean/paper/1202_2/0_3.png}
	}%
	\subfloat[]{%
		\includegraphics[width=0.185\linewidth]{figs/results/appendix/texture_transfer/img/1202_3/seg.png}
	}%

	\vspace{-0.8cm}%

	\subfloat[]{%
		\includegraphics[width=0.185\linewidth]{figs/results/appendix/texture_transfer/img/1203_4/img.png}
	}%
	\subfloat[]{%
		\includegraphics[width=0.185\linewidth]{figs/results/appendix/texture_transfer/img/1203_3/img.png}
	}%
	\subfloat[]{%
		\includegraphics[width=0.185\linewidth]{figs/results/appendix/texture_transfer/replace/paper/1203_3/0_4.png}
	}%
	\subfloat[]{%
		\includegraphics[width=0.185\linewidth]{figs/results/appendix/texture_transfer/mean/paper/1203_3/0_4.png}
	}%
	\subfloat[]{%
		\includegraphics[width=0.185\linewidth]{figs/results/appendix/texture_transfer/img/1203_4/seg.png}
	}%

\vspace{-0.8cm}%

	\subfloat[]{%
		\includegraphics[width=0.185\linewidth]{figs/results/appendix/texture_transfer/img/1204_3/img.png}
	}%
	\subfloat[]{%
		\includegraphics[width=0.185\linewidth]{figs/results/appendix/texture_transfer/img/1204_1/img.png}
	}%
	\subfloat[]{%
		\includegraphics[width=0.185\linewidth]{figs/results/appendix/texture_transfer/replace/paper/1204_1/0_3.png}
	}%
	\subfloat[]{%
		\includegraphics[width=0.185\linewidth]{figs/results/appendix/texture_transfer/mean/paper/1204_1/0_3.png}
	}%
	\subfloat[]{%
		\includegraphics[width=0.185\linewidth]{figs/results/appendix/texture_transfer/img/1204_3/seg.png}
	}%

	\vspace{-0.8cm}%
	
	\subfloat[Structure]{%
		\includegraphics[width=0.185\linewidth]{figs/results/appendix/texture_transfer/img/1204_6/img.png}
	}%
	\subfloat[Appearance]{%
		\includegraphics[width=0.185\linewidth]{figs/results/appendix/texture_transfer/img/1204_7/img.png}
	}%
	\subfloat[Replacement]{%
		\includegraphics[width=0.185\linewidth]{figs/results/appendix/texture_transfer/replace/paper/1204_7/0_6.png}
	}%
	\subfloat[Mean alignment (default)]{%
		\includegraphics[width=0.185\linewidth]{figs/results/appendix/texture_transfer/mean/paper/1204_7/0_6.png}
	}%
	\subfloat[Seg. overlay]{%
		\includegraphics[width=0.185\linewidth]{figs/results/appendix/texture_transfer/img/1204_6/seg.png}
	}	

	\Caption{Two texture transfer mechanisms.}{
		Segmentations of the structure-providing textures are displayed on the right.
	}
	\label{fig:texture_transfer_mechanism}
\end{figure*}
