# Supplementary material for: Compositional Neural Textures
Source: arXiv:2404.12509 source file (2024-09-23)
Supplement: Supplementary file 5 [file appendix.tex]

\section{Appendix}
