# Supplementary material for: Compositional Neural Textures
Source: arXiv:2404.12509 source file (2024-09-23)
Supplement: Supplementary file 6 [file fig_appendix_ablation_losses0.tex]

\begin{figure*}[b]
	\centering
	\captionsetup[subfigure]{labelformat=empty}
	\begingroup
	\setlength{\tabcolsep}{-2pt} 
	
	\begin{tabular}{ccccccccc}
		\subfloat[Input]{
			\includegraphics[width=0.11\linewidth]{figs/results/ablations/01112024/full/img/300_5/img.png}
		}&
		\subfloat[]{
			\raisebox{0.3in}{\rotatebox[origin=t]{90}{Seg. Overlay}}
		}
		&
		\subfloat[]{
			\includegraphics[width=0.11\linewidth]{figs/results/ablations/01112024/nocompact/img/300_5/seg.png}
		}&
		\subfloat[]{
			\includegraphics[width=0.11\linewidth]{figs/results/ablations/01112024/noentropy/img/300_5/seg.png}
		}&
		\subfloat[]{
			\includegraphics[width=0.11\linewidth]{figs/results/ablations/01112024/noconsist/img/300_5/seg.png}
		}&
		\subfloat[]{
			\includegraphics[width=0.11\linewidth]{figs/results/ablations/01112024/notexture/img/300_5/seg.png}
		}&
		\subfloat[]{
		\includegraphics[width=0.11\linewidth]{figs/results/ablations/01112024/nogan/img/300_5/seg.png}
		}&
		\subfloat[]{
		\includegraphics[width=0.11\linewidth]{figs/results/ablations/01112024/nopgan/img/300_5/seg.png}
		}&
		\subfloat[]{
		\includegraphics[width=0.11\linewidth]{figs/results/ablations/01112024/full/img/300_5/seg.png}
		}\\[-0.825cm]
		&
		\subfloat[]{
			\raisebox{0.3in}{\rotatebox[origin=t]{90}{Gaussians}}
		}
		&
		\subfloat[]{
			\includegraphics[width=0.11\linewidth]{figs/results/ablations/01112024/nocompact/img/300_5/gaussian.png}
		}&
		\subfloat[]{
			\includegraphics[width=0.11\linewidth]{figs/results/ablations/01112024/noentropy/img/300_5/gaussian.png}
		}&
		\subfloat[]{
			\includegraphics[width=0.11\linewidth]{figs/results/ablations/01112024/noconsist/img/300_5/gaussian.png}
		}&
		\subfloat[]{
			\includegraphics[width=0.11\linewidth]{figs/results/ablations/01112024/notexture/img/300_5/gaussian.png}
		}&
		\subfloat[]{
			\includegraphics[width=0.11\linewidth]{figs/results/ablations/01112024/nogan/img/300_5/gaussian.png}
		}&
		\subfloat[]{
			\includegraphics[width=0.11\linewidth]{figs/results/ablations/01112024/nopgan/img/300_5/gaussian.png}
		}&
		\subfloat[]{
			\includegraphics[width=0.11\linewidth]{figs/results/ablations/01112024/full/img/300_5/gaussian.png}
		}\\[-0.825cm]
		&
		\subfloat[]{
		\raisebox{0.3in}{
			\rotatebox[origin=t]{90}{
					Recon.
			}
		} 
	}
		&
		\subfloat[]{
		\includegraphics[width=0.11\linewidth]{figs/results/ablations/01112024/nocompact/img/300_5/recon.png}
		}&
		\subfloat[]{
			\includegraphics[width=0.11\linewidth]{figs/results/ablations/01112024/noentropy/img/300_5/recon.png}
		}&
		\subfloat[]{
			\includegraphics[width=0.11\linewidth]{figs/results/ablations/01112024/noconsist/img/300_5/recon.png}
		}&
		\subfloat[]{
			\includegraphics[width=0.11\linewidth]{figs/results/ablations/01112024/notexture/img/300_5/recon.png}
		}&
		\subfloat[]{
			\includegraphics[width=0.11\linewidth]{figs/results/ablations/01112024/nogan/img/300_5/recon.png}
		}&
		\subfloat[]{
			\includegraphics[width=0.11\linewidth]{figs/results/ablations/01112024/nopgan/img/300_5/recon.png}
		}&
		\subfloat[]{
			\includegraphics[width=0.11\linewidth]{figs/results/ablations/01112024/full/img/300_5/recon.png}
		}\\[-0.825cm]
		\subfloat[]{%
			\includegraphics[width=0.11\linewidth]{figs/results/ablations/01112024/full/300_0/texture.png}%
		}%
		&
		\raisebox{8ex}{
		\multirow{2}{*}{
			\subfloat[]{
				\raisebox{-1.5ex}{
					\rotatebox[origin=t]{90}{
						Texture Transfer
					}
				} 
			}
		}%
		}%
		&
		\subfloat[]{
			\includegraphics[width=0.11\linewidth]{figs/results/ablations/01112024/nocompact/300_0/0_5.png}
		}&
		\subfloat[]{
			\includegraphics[width=0.11\linewidth]{figs/results/ablations/01112024/noentropy/300_0/0_5.png}
		}&
		\subfloat[]{
			\includegraphics[width=0.11\linewidth]{figs/results/ablations/01112024/noconsist/300_0/0_5.png}
		}&
		\subfloat[]{
			\includegraphics[width=0.11\linewidth]{figs/results/ablations/01112024/notexture/300_0/0_5.png}
		}&
		\subfloat[]{
			\includegraphics[width=0.11\linewidth]{figs/results/ablations/01112024/nogan/300_0/0_5.png}
		}&
		\subfloat[]{
			\includegraphics[width=0.11\linewidth]{figs/results/ablations/01112024/nopgan/300_0/0_5.png}
		}&
		\subfloat[]{
			\includegraphics[width=0.11\linewidth]{figs/results/ablations/01112024/full/300_0/0_5.png}
		}\\[-0.825cm]
		\subfloat[Appearance]{%
			\includegraphics[width=0.11\linewidth]{figs/results/ablations/01112024/full/300_6/texture.png}%
		}%
		&

		&
		\subfloat[]{
			\includegraphics[width=0.11\linewidth]{figs/results/ablations/01112024/nocompact/300_6/0_5.png}
		}&
		\subfloat[]{
			\includegraphics[width=0.11\linewidth]{figs/results/ablations/01112024/noentropy/300_6/0_5.png}
		}&
		\subfloat[]{
			\includegraphics[width=0.11\linewidth]{figs/results/ablations/01112024/noconsist/300_6/0_5.png}
		}&
		\subfloat[]{
			\includegraphics[width=0.11\linewidth]{figs/results/ablations/01112024/notexture/300_6/0_5.png}
		}&
		\subfloat[]{
			\includegraphics[width=0.11\linewidth]{figs/results/ablations/01112024/nogan/300_6/0_5.png}
		}&
		\subfloat[]{
			\includegraphics[width=0.11\linewidth]{figs/results/ablations/01112024/nopgan/300_6/0_5.png}
		}&
		\subfloat[]{
			\includegraphics[width=0.11\linewidth]{figs/results/ablations/01112024/full/300_6/0_5.png}
		}\\[-0.4cm]
		\subfloat[Input]{
			\includegraphics[width=0.11\linewidth]{figs/results/ablations/01112024/full/img/300_10/img.png}
		}&
		\subfloat[]{
			\raisebox{0.3in}{\rotatebox[origin=t]{90}{Seg. Overlay}}
		}
		&
		\subfloat[]{
			\includegraphics[width=0.11\linewidth]{figs/results/ablations/01112024/nocompact/img/300_10/seg.png}
		}&
		\subfloat[]{
			\includegraphics[width=0.11\linewidth]{figs/results/ablations/01112024/noentropy/img/300_10/seg.png}
		}&
		\subfloat[]{
			\includegraphics[width=0.11\linewidth]{figs/results/ablations/01112024/noconsist/img/300_10/seg.png}
		}&
		\subfloat[]{
			\includegraphics[width=0.11\linewidth]{figs/results/ablations/01112024/notexture/img/300_10/seg.png}
		}&
		\subfloat[]{
		\includegraphics[width=0.11\linewidth]{figs/results/ablations/01112024/nogan/img/300_10/seg.png}
		}&
		\subfloat[]{
		\includegraphics[width=0.11\linewidth]{figs/results/ablations/01112024/nopgan/img/300_10/seg.png}
		}&
		\subfloat[]{
		\includegraphics[width=0.11\linewidth]{figs/results/ablations/01112024/full/img/300_10/seg.png}
		}\\[-0.825cm]
		&
		\subfloat[]{
			\raisebox{0.3in}{\rotatebox[origin=t]{90}{Gaussians}}
		}
		&
		\subfloat[]{
			\includegraphics[width=0.11\linewidth]{figs/results/ablations/01112024/nocompact/img/300_10/gaussian.png}
		}&
		\subfloat[]{
			\includegraphics[width=0.11\linewidth]{figs/results/ablations/01112024/noentropy/img/300_10/gaussian.png}
		}&
		\subfloat[]{
			\includegraphics[width=0.11\linewidth]{figs/results/ablations/01112024/noconsist/img/300_10/gaussian.png}
		}&
		\subfloat[]{
			\includegraphics[width=0.11\linewidth]{figs/results/ablations/01112024/notexture/img/300_10/gaussian.png}
		}&
		\subfloat[]{
			\includegraphics[width=0.11\linewidth]{figs/results/ablations/01112024/nogan/img/300_10/gaussian.png}
		}&
		\subfloat[]{
			\includegraphics[width=0.11\linewidth]{figs/results/ablations/01112024/nopgan/img/300_10/gaussian.png}
		}&
		\subfloat[]{
			\includegraphics[width=0.11\linewidth]{figs/results/ablations/01112024/full/img/300_10/gaussian.png}
		}\\[-0.825cm]
		&
		\subfloat[]{
		\raisebox{0.3in}{
			\rotatebox[origin=t]{90}{
					Recon.
			}
		} 
	}
		&
		\subfloat[]{
		\includegraphics[width=0.11\linewidth]{figs/results/ablations/01112024/nocompact/img/300_10/recon.png}
		}&
		\subfloat[]{
			\includegraphics[width=0.11\linewidth]{figs/results/ablations/01112024/noentropy/img/300_10/recon.png}
		}&
		\subfloat[]{
			\includegraphics[width=0.11\linewidth]{figs/results/ablations/01112024/noconsist/img/300_10/recon.png}
		}&
		\subfloat[]{
			\includegraphics[width=0.11\linewidth]{figs/results/ablations/01112024/notexture/img/300_10/recon.png}
		}&
		\subfloat[]{
			\includegraphics[width=0.11\linewidth]{figs/results/ablations/01112024/nogan/img/300_10/recon.png}
		}&
		\subfloat[]{
			\includegraphics[width=0.11\linewidth]{figs/results/ablations/01112024/nopgan/img/300_10/recon.png}
		}&
		\subfloat[]{
			\includegraphics[width=0.11\linewidth]{figs/results/ablations/01112024/full/img/300_10/recon.png}
		}\\[-0.825cm]
		\subfloat[]{%
			\includegraphics[width=0.11\linewidth]{figs/results/ablations/01112024/full/300_0/texture.png}%
		}%
		&
		\raisebox{8ex}{
		\multirow{2}{*}{
			\subfloat[]{
				\raisebox{-1.5ex}{
					\rotatebox[origin=t]{90}{
						Texture Transfer
					}
				} 
			}
		}%
		}%
		&
		\subfloat[]{
			\includegraphics[width=0.11\linewidth]{figs/results/ablations/01112024/nocompact/300_0/0_10.png}
		}&
		\subfloat[]{
			\includegraphics[width=0.11\linewidth]{figs/results/ablations/01112024/noentropy/300_0/0_10.png}
		}&
		\subfloat[]{
			\includegraphics[width=0.11\linewidth]{figs/results/ablations/01112024/noconsist/300_0/0_10.png}
		}&
		\subfloat[]{
			\includegraphics[width=0.11\linewidth]{figs/results/ablations/01112024/notexture/300_0/0_10.png}
		}&
		\subfloat[]{
			\includegraphics[width=0.11\linewidth]{figs/results/ablations/01112024/nogan/300_0/0_10.png}
		}&
		\subfloat[]{
			\includegraphics[width=0.11\linewidth]{figs/results/ablations/01112024/nopgan/300_0/0_10.png}
		}&
		\subfloat[]{
			\includegraphics[width=0.11\linewidth]{figs/results/ablations/01112024/full/300_0/0_10.png}
		}\\[-0.825cm]
		\subfloat[Appearance]{%
			\includegraphics[width=0.11\linewidth]{figs/results/ablations/01112024/full/300_6/texture.png}%
		}%
		&

		&
		\subfloat[w/o $\losscompact$]{
			\includegraphics[width=0.11\linewidth]{figs/results/ablations/01112024/nocompact/300_6/0_10.png}
		}&
		\subfloat[w/o $\lossentropy$]{
			\includegraphics[width=0.11\linewidth]{figs/results/ablations/01112024/noentropy/300_6/0_10.png}
		}&
		\subfloat[w/o $\lossmatch$]{
			\includegraphics[width=0.11\linewidth]{figs/results/ablations/01112024/noconsist/300_6/0_10.png}
		}&
		\subfloat[w/o $\losstexture$]{
			\includegraphics[width=0.11\linewidth]{figs/results/ablations/01112024/notexture/300_6/0_10.png}
		}&
		\subfloat[w/o $\lossgan$]{
			\includegraphics[width=0.11\linewidth]{figs/results/ablations/01112024/nogan/300_6/0_10.png}
		}&
		\subfloat[w/o $\losspatchgan$]{
			\includegraphics[width=0.11\linewidth]{figs/results/ablations/01112024/nopgan/300_6/0_10.png}
		}&
		\subfloat[Full]{
			\includegraphics[width=0.11\linewidth]{figs/results/ablations/01112024/full/300_6/0_10.png}
		}%
	\end{tabular}
	\endgroup
	\Caption{Continuation of \Cref{fig:ablation_studies}.}{%
	}
	\label{fig:appendix:ablation_losses0}
\end{figure*}
