# Supplementary material for: Compositional Neural Textures
Source: arXiv:2404.12509 source file (2024-09-23)
Supplement: Supplementary file 7 [file fig_appendix_additional_results_segmentation.tex]

\begin{figure*}[b]

    \centering
    \captionsetup[subfigure]{labelformat=empty}

    \newcounter{mycounter1}
    \setcounter{mycounter1}{0} %

    \foreach \b in {100,...,104}{%
        \foreach \i in {12,...,17}{
            \includegraphics[width=0.095\linewidth]{figs/results/appendix/texton_segmentation/img/\b_\i.png}%
            \includegraphics[width=0.095\linewidth]{figs/results/appendix/texton_segmentation/seg/\b_\i.png}%
            \addtocounter{mycounter1}{1}
        }
        \ifnum\value{mycounter1}=5
            \setcounter{mycounter1}{0} 
            \\
        \fi
    }%
    \foreach \b in {105,...,107}{%
        \foreach \i in {0,...,9}{
            \includegraphics[width=0.095\linewidth]{figs/results/appendix/texton_segmentation/img/\b_\i.png}%
            \includegraphics[width=0.095\linewidth]{figs/results/appendix/texton_segmentation/seg/\b_\i.png}%
            \addtocounter{mycounter1}{1}
        }
        \ifnum\value{mycounter1}=5
            \setcounter{mycounter1}{0} 
            \\
        \fi
    }%

    \Caption{Continuation from \Cref{fig:results_segmentation}.}
    {%
        
    }
    \label{fig:additional_results_segmentation}
\end{figure*}
