# Supplementary material for: Compositional Neural Textures
Source: arXiv:2404.12509 source file (2024-09-23)
Supplement: Supplementary file 8 [file fig_appendix_comparison_segmentation.tex]

\begin{figure*}[b]
	\centering
	\captionsetup[subfigure]{labelformat=empty}

	\newcounter{seg_comparison_counter}
    \setcounter{seg_comparison_counter}{0} %

	\foreach \b in {110,...,111}{%
		\foreach \i in {0,...,17}{
			\includegraphics[width=0.095\linewidth]{figs/results/appendix/texton_segmentation/img/\b_\i.png}%
			\includegraphics[width=0.095\linewidth]{figs/results/appendix/texton_segmentation/sa/img_seg_\b_\i.png}%
			\includegraphics[width=0.095\linewidth]{figs/results/appendix/texton_segmentation/seg/\b_\i.png}%
			\addtocounter{seg_comparison_counter}{1}%
		}
		\ifnum\value{seg_comparison_counter}=3
			\setcounter{seg_comparison_counter}{0} 
			\\[-2ex]
		\fi
	}%
	\Caption{Uncurated comparisons with SA.}%
	{%
	Each set contains 3 images:
	the input (left),
	result from SA \cite{Meta:2023:SA} trained with 1 billion masks (middle),
	and our model's output (right).
	Notably, despite SA's reliance on extensive supervision, our model successfully extracts textons without supervision.
	}
	\label{fig:appendix:comparison_segment}
\end{figure*}
