# Supplementary material for: Compositional Neural Textures
Source: arXiv:2404.12509 source file (2024-09-23)
Supplement: Supplementary file 10 [file fig_appendix_comparison_transfer1.tex]

\begin{figure*}[b]
    
\centering
\captionsetup[subfigure]{labelformat=empty}

\input{figs/results/comparisons/texture_transfer/current/visual_1.txt}%

\Caption{Continuation from \Cref{fig:appendix:comparison_transfer}.}
{
}
\label{fig:appendix:additional_comparison_transfer}
    
\end{figure*}
