# Supplementary material for: Compositional Neural Textures
Source: arXiv:2404.12509 source file (2024-09-23)
Supplement: Supplementary file 11 [file fig_appendix_dataset_samples.tex]

\begin{figure}[h]

    \centering
    \captionsetup[subfigure]{labelformat=empty}
    
        \foreach \n in {0,...,4}{
            \includegraphics[width=0.19\linewidth]{figs/results/appendix/data_samples/\n.png}%
        }
    
        \foreach \n in {5,...,9}{
            \includegraphics[width=0.19\linewidth]{figs/results/appendix/data_samples/\n.png}%
        }
    
        \foreach \n in {10,...,14}{
            \includegraphics[width=0.19\linewidth]{figs/results/appendix/data_samples/\n.png}%
        }
    
        \foreach \n in {15,...,19}{
            \includegraphics[width=0.19\linewidth]{figs/results/appendix/data_samples/\n.png}%
        }
    
        \foreach \n in {20,...,24}{
            \includegraphics[width=0.19\linewidth]{figs/results/appendix/data_samples/\n.png}%
        }
    
        \foreach \n in {25,...,29}{
            \includegraphics[width=0.19\linewidth]{figs/results/appendix/data_samples/\n.png}%
        }
    
        \foreach \n in {30,...,34}{
            \includegraphics[width=0.19\linewidth]{figs/results/appendix/data_samples/\n.png}%
        }

    \Caption{100 original dataset samples without augmentation.}
    {%
        
    }
    \label{fig:dataset_samples}
    \end{figure}
