# Supplementary material for: Compositional Neural Textures
Source: arXiv:2404.12509 source file (2024-09-23)
Supplement: Supplementary file 13 [file fig_appendix_uncurated_comparison_transfer0.tex]

\begin{figure*}[b]
    
    \centering
    \captionsetup[subfigure]{labelformat=empty}
    
    \input{figs/results/comparisons/texture_transfer/current/user_0.txt}%

\Caption{Uncurated comparisons with \replace{state-of-the-art}{existing} approaches on texture transfer.}
{

}
\label{fig:appendix:uncurated_comparison_transfer0}
    
\end{figure*}
