# Supplementary material for: Compositional Neural Textures
Source: arXiv:2404.12509 source file (2024-09-23)
Supplement: Supplementary file 16 [file fig_appendix_uncurated_comparison_transfer3.tex]

\begin{figure*}[b]
    
    \centering
    \captionsetup[subfigure]{labelformat=empty}
    
    \input{figs/results/comparisons/texture_transfer/current/user_3.txt}%

\Caption{Continuation from \Cref{fig:appendix:uncurated_comparison_transfer0}.}
{

}
\label{fig:appendix:uncurated_comparison_transfer3}
    
\end{figure*}
